# Supplementary material for: Enhancing Gradient Inversion Attacks in Federated Learning via Hierarchical Feature Optimization
Source: arXiv:2604.00955 source file (2026-11-07)
Supplement: Supplementary file 1 [file appendix-attack.tex]

\section{Inversion Attack for NIDS}
\label{inversion_attack_appendix}
We present optimization-based inversion attack designed for NIDS in algorithm \ref{algorithm_inversion}.
We adapt Adam optimizer to search for the optimal reconstructed data and label with different distance metric (lines 5-7) according to different scenarios.
To further preserve the functionality of the reconstructed data, we project $x^*$ into legal feature space (line 12) and set the corresponding original discrete features to integers (lines 13-17).

\begin{algorithm}
    \caption{Optimization-based inversion attack}
    \label{algorithm_inversion}
    \KwIn{user's shared gradient $\nabla \theta(x,y)$, local user's loss function $\ell$ on differentiable model, attack epochs $recon\_iters$, learning rate $\alpha$, distance metric $attack\_type$, maximum/minimum range of data $x_{max}/x_{min}$, batch size $bs$, discrete features index $discrete\_index$}
    \KwOut{reconstructed private data $x^*$ and label $y^*$} 
    $x^*\leftarrow U(0, 1), y^*\leftarrow U(0, 1)$; \Comment{random initialization}\\
    \For{$k \leftarrow 1$ to $bs$}
    {\For {$i\leftarrow1$ to $recon\_iters$} 
    {$\nabla \theta(x^*,y^*) \leftarrow \frac{\partial\ell(\theta, x^*, y^*)}{\partial \theta}$; \Comment{dummy gradient computation}\\
    \lIf{$attack\_type==L_2$}{$loss\leftarrow \Vert\nabla \theta(x^*,y^*)-\nabla \theta(x,y)\Vert_2$}\Comment{choose distance metric}\\ \lElse{$loss\leftarrow 1-\frac{\langle \nabla \theta(x^*,y^*),\nabla \theta(x,y) \rangle }{\Vert\nabla \theta(x^*,y^*)\Vert\Vert\nabla \theta(x,y)\Vert}$}
    $x_k^* \leftarrow Adam(x_k^*, \frac{\partial loss}{\partial x_k^*}, \alpha)$; \Comment{Adam optimizer}\\
    $y_k^* \leftarrow Adam(y_k^*, \frac{\partial loss}{\partial y_k^*}, \alpha)$\;
    }}
    $x^* \leftarrow clamp(x^*, min=0, max=1)$\;
    $x^* \leftarrow x^*(x_{max}-x_{min})+x_{min}$\;
    \For{each discrete index i in $discrete\_index$}
    {$x^*_i \leftarrow round(x^*_i$)}
    $x^* \leftarrow \frac{x^*-x_{min}}{x_{max}-x_{min}},\ \ y^* \leftarrow argmax(y^*)$\;
    \textbf{return} $x^*, y^*$
\end{algorithm}
