# Supplementary material for: Enhancing Gradient Inversion Attacks in Federated Learning via Hierarchical Feature Optimization
Source: arXiv:2604.00955 source file (2026-11-07)
Supplement: Supplementary file 3 [file appendix.tex]

\documentclass[journal]{IEEEtran}
\usepackage{amsmath,amsfonts}
\usepackage{algorithm}
\usepackage{array}
\usepackage{textcomp}
\usepackage{stfloats}
\usepackage{url}
\usepackage{verbatim}
\usepackage{graphicx}
\usepackage{cite}
\usepackage{amsmath,amssymb,amsfonts,amsthm,bm}
\usepackage{algorithmicx}
\usepackage{algpseudocode}
\usepackage{support-caption}
\usepackage{subcaption}
\usepackage{graphicx}
\usepackage{longtable}
\usepackage{multirow}
\usepackage{tabularx}
\usepackage{booktabs}
\usepackage{textcomp}
\usepackage{stfloats}
\usepackage{url}
\usepackage{verbatim}
\usepackage{graphicx}
\usepackage{color}
\usepackage[acronyms]{glossaries}

\algnewcommand\algorithmicinput{\textbf{Input:}}
\algnewcommand\algorithmicoutput{\textbf{Output:}}
\algnewcommand\INPUT{\item[\algorithmicinput]} 
\algnewcommand\OUTPUT{\item[\algorithmicoutput]}

\hyphenation{op-tical net-works semi-conduc-tor IEEE-Xplore}

\usepackage[hidelinks]{hyperref}

\usepackage{enumitem}

\newacronym{sbl}{SBL}{sparse Bayesian learning}
\newacronym{ml}{ML}{maximum likelihood}
\newacronym{pdf}{PDF}{probability density function}
\newacronym{snr}{SNR}{signal-to-noise ratio}
\newacronym{em}{EM}{expectation-maximization}
\newacronym{awgn}{AWGN}{additive white Gaussian noise}
\newacronym{nmse}{NMSE}{normalized mean squared error}
\newacronym{mmse}{MMSE} {minimum mean squared error}
\newacronym{elbo}{ELBO}{evidence lower bound}
\newacronym{kl}{KL}{Kullback-Leibler}

\begin{document}

\title{Enhancing Gradient Inversion Attacks in Federated Learning via Hierarchical Feature Optimization}

    \author{Hao Fang$^*$,
    Wenbo Yu$^*$,
    Bin Chen$^{\dagger}$,~\IEEEmembership{Member,~IEEE,}
    Xuan Wang,~\IEEEmembership{Member,~IEEE,}\\
    % Zhi Wang,~\IEEEmembership{Senior Member,~IEEE,}
    Shu-Tao Xia,~\IEEEmembership{ Member,~IEEE,}
    Qing Liao,~\IEEEmembership{Member,~IEEE,}
    Ke Xu,~\IEEEmembership{Fellow,~IEEE}
}

\maketitle
\setcounter{section}{0}
\renewcommand{\thesection}{\Alph{section}}

\section{Details about Gradient Transformation}
\label{sec:details}
To handle the potentially applied defense mechanisms, the adversary can infer three defense approaches as follows (denote the received gradients by $g$):

(1) \textit{Gradient clipping.} Given a clipping bound $c$, gradient clipping transforms the gradients as $\mathcal{T}(g,c) = g\cdot\min(\frac{c}{\Vert g\Vert_2},1)$. Since this operation is always layer-wise, the attacker can compute the $\ell_2$ norm at each layer of the received gradients as the estimated clipping bound.

(2) \textit{Gradient sparsification.} Given a pruning rate $p\in(0,1)$, the client only transmits the $(1 - p)$ largest values of $g$ (in absolute value) and the rest values are replaced by zero. Implemented by applying a layer-wise mask, the gradient sparsity can be estimated by observing the percentage of non-zero entries in the shared gradients.

(3) \textit{Soteria.} Recently proposed by \cite{sun2021soteria}, it is an efficient and reliable defense strategy. This operation is actually equivalent to applying a mask only to the gradients of the defended layer. Once the global model $f_\theta$ and input $\mathbf{x}$ are given, this process becomes deterministic. Then, the attacker can invert this mask according to the non-zero entries of the gradients from the defended layer.

\section{Radius Hyperparameter Setting}
\label{sec:experi_details}

Guided by the theory \cite{daras2021intermediate} that a sequence of increasing radii of the $l_1$ ball tends to provide better results, we gradually allow larger deviations and tune the $r$ by experiment, obtaining an appropriate setting as follows.

(1) For BigGAN, we constrain the intermediate features:
\begin{itemize}
    \item Intermediate features: [2000, 2500, 3000, 3500, 4000, 4500, 5000, 5500, 6000]. 
\end{itemize}

(2) In addition to the intermediate features, StyleGAN2 has more particularities we need to handle for feature domain optimization. Specifically, we optimize the noise vectors and apply the $l_1$ ball constraint to them at the same time. Involved in the generation of styles in StyleGAN2, the latent vectors also need to be optimized, and we constrain their searching range within an $l_1$ ball as well:
\begin{itemize}
    \item Intermediate features: [2000, 3000, 4000, 5000]
    \item Noises: [1000, 2000, 3000, 4000, 5000]
    \item Latent vectors: [1000, 2000, 3000, 4000, 5000]
\end{itemize}

\bibliographystyle{IEEEtran}
\bibliography{Bibliography}

\end{document}
